# Supplementary material for: Switch-KD: Visual-Switch Knowledge Distillation for Vision-Language Models
Source: arXiv:2604.14629 source file (2026-04-16)
Supplement: Supplementary file 1 [file X_suppl.tex]

\clearpage
\setcounter{page}{1}
\maketitlesupplementary

\setcounter{section}{0}

\section*{Supplementary Overview}
\addcontentsline{toc}{section}{Supplementary Overview}
% \noindent The following provides an overview of the content in each Appendix section:
This supplementary material provides an overview of the content in each appendix section:
\begin{itemize}
    \item \textbf{Section A}: Extended Background and Related Work.
    \item \textbf{Section B}: Additional Implement Details. 
    \item \textbf{Section C}: Comparison with SOTA Distilled VLMs
    \item \textbf{Section D}: More Ablation and Explanatory Analysis.
    \item \textbf{Section E}: Detailed Results.
\end{itemize}

% \section{Additional Related Work}
\section{Extended Background and Related Work}
\label{sec:relatedwork}
% We first provide a more comprehensive review of related work beyond the brief discussion, covering key developments in large and lightweight vision–language models.
We present a more comprehensive review of related work, expanding upon the brief discussion and focusing on advances in large and lightweight vision–language models.

\paragraph{Large Vision-Language Models:~}
% \subsection{Large Vision-Language Models}
% \label{method:lvlm}
Recent advances in large vision-language models (VLMs) have led to significant progress in visual-language understanding. 
Early methods, such as CLIP \cite{radford2021learning}, typically relied on contrastive learning over roughly 400 million image–text pairs to establish alignment between visual and textual modalities.
%Early methods—for example, CLIP \cite{radford2021learning} often trained on approximately 400 million image-text pairs using contrastive learning to establish alignment between visual and textual modalities. 
Subsequently, models such as BLIP‑2 \cite{li2023blip} adopted a paradigm of integrating a frozen pretrained vision encoder with a large language model (LLM), and introduced a lightweight Q-Former bridging module to enable multimodal understanding and generation. More recently, research \cite{liu2023visual,bai2023qwen,wang2025internvl3_5} has largely adopted the architecture of ViT–Projector–LLM, and applied instruction tuning to enable multimodal dialogue and reasoning capabilities. 
Regarding the performance improvements of large VLMs, numerous studies \cite{kumar2024scaling,nezhurina2025scaling,peng2025scaling} show that their gains roughly follow the scaling law observed in language models. As model size, training data, and compute increase, performance typically improves.
%Regarding the performance improvements of large VLMs, numerous studies \cite{kumar2024scaling,nezhurina2025scaling,peng2025scaling} indicate their gains roughly follow the “scaling law” observed in language models — namely that as model size, training data volume, and compute budget increase, performance typically improves; however, the marginal returns diminish as scale grows further. 
Nevertheless, in resource-constrained or real-time deployment scenarios, these large VLMs face serious bottlenecks in terms of compute resource requirements, storage footprint, and inference latency, making lightweight alternatives particularly necessary.

% \textbf{Lightweight Vision-Language Models.}
% \subsection{Lightweight Vision-Language Models}
\paragraph{Lightweight Vision-Language Models:~}
\label{method:lightvlm}
Recently, researchers \cite{zhou2024tinyllava,li2024mini,liu2024sphinx,chu2024mobilevlm} have proposed a series of lightweight vision-language model frameworks from three perspectives: architecture design, data quality, and training strategy.
TinyLLaVA~\cite{zhou2024tinyllava} introduces compact LLM backbones and efficient fine-tuning strategies, achieving performance comparable to 7B-scale models within only 1B–3B parameters.
Mini-Gemini~\cite{li2024mini} adopts a dual-visual-encoder design and a patch information mining mechanism to effectively integrate fine-grained details from high-resolution images while maintaining low computational cost.
SPHINX-X~\cite{liu2024sphinx} further streamlines the visual encoder design, incorporates skip tokens for architectural efficiency, and adopts a unified one-stage training scheme that facilitates more efficient deployment.
% MobileVLM V2 \cite{chu2024mobilevlm} leverages the lightweight LDPv2 projector, a high-quality 3.6M dataset, and a full-LLM training strategy during pre-training, resulting in notably stronger overall performance and achieving the fastest inference speed among models of similar scale on mobile devices.
MobileVLM V2~\cite{chu2024mobilevlm} employs the lightweight LDPv2 projector, a high-quality 3.6M dataset, and a full-LLM pre-training strategy, achieving higher benchmark accuracy and the fastest inference speed among similarly scaled models on mobile devices.

\section{Additional Implement Details}
\label{sec:implement}
\begin{table}[htbp]
\centering
\begin{tabular}{c|cl}
\toprule
\textbf{Training Phase} & \textbf{Task} & \textbf{Datasets (\# Size)} \\
\midrule
\textbf{PT} & Caption & LCS (558K) \\
\midrule
\multirow{10}{*}{\textbf{SFT / DFT}} 
& \multirow{4}{*}{VQA} 
& VQAv2 (83K) \\
& & GQA (72K) \\
& & OKVQA (9K) \\
& & A-OKVQA (50K) \\
\cmidrule{2-3}
& \multirow{2}{*}{OCR}
& OCRVQA (80K) \\
& & TextCaps (22K) \\
\cmidrule{2-3}
& \multirow{2}{*}{Region} 
&  RefCOCO (30K) \\
& & VG (86K) \\
\cmidrule{2-3}
& \multirow{2}{*}{Conversation}  
& LLaVA (158K) \\
& & ShareGPT (40K) \\
\midrule
\textbf{Total} &  & \textbf{1.2M} \\
\bottomrule
\end{tabular}
\caption{Dataset composition for each training phase.}
\label{tab:dataset_composition}
\end{table}
\paragraph{Training datasets. }
Table~\ref{tab:dataset_composition} summarizes the dataset composition across different training phases. 
The pretraining dataset LCS-558K consists of 558k image–text pairs from LAION-CC-SBU, annotated with BLIP captions. 
The 665k instruction-following dataset includes a diverse collection of tasks: 
VQA~\cite{goyal2017making, hudson2019gqa, marino2019ok, schwenk2022okvqa}, 
OCR~\cite{mishra2019ocr, sidorov2020textcaps}, 
region-level VQA~\cite{kazemzadeh2014referitgame, krishna2017visual, mao2016generation}, 
visual conversation~\cite{liu2023visual}, 
and general language conversation data.

\begin{table}[htbp]
\centering
\begin{tabular}{lcc}
\toprule
\textbf{Hyperparameter} & \textbf{PT} & \textbf{DFT} \\
\midrule
Visual Encoder  & $\times$ & \checkmark \\
Projector       & \checkmark & \checkmark \\
LLM             & $\times$ & \checkmark \\
\midrule
Image Resolution    & \multicolumn{2}{c}{384$\times$384} \\
Learning Rate       & 1e-3 & 2e-5 \\
Optimizer           & \multicolumn{2}{c}{AdamW} \\
Scheduler           & \multicolumn{2}{c}{Cosine decay} \\
Warm up ratio       & \multicolumn{2}{c}{0.03} \\
Global Batch Size   & 256 & 128 \\
Epoch               & \multicolumn{2}{c}{1} \\
DeepSpeed stage     & Zero 2 & Zero 2 \\
\bottomrule
\end{tabular}
\caption{Hyperparameters of Switch-KD.}
\label{tab:hparams}
\end{table}

\paragraph{Training Hyperparameters.~}
We adopt a similar set of hyperparameters to those used in LLaVA-KD. 
The configurations for the first-stage vision–language alignment pretraining and the second-stage distillation-based instruction tuning are summarized in Table~\ref{tab:hparams}.

% \section{Pseudocode For Method}
% \subsection{Pseudocode For Method}
\paragraph{Pseudocode for the Proposed Method.~}
For clarity and reproducibility, we present pseudo-code illustrating the implementation of our \emph{Visual-Switch Distillation} framework and its core \emph{DBiLD Loss} in Algorithm~\ref{alg:vsd} and Algorithm~\ref{alg:dbild_calc}, respectively. 
The first algorithm outlines the overall visual-switch distillation process, while the second specifies the dynamic bidirectional logits alignment procedure. 
%All experiments are conducted under the hyperparameter settings summarized in Table~\ref{tab:hparams}.

\begin{algorithm}[htbp]
\caption{Visual-Switch Distillation}
\label{alg:vsd}
\begin{flushleft}
\textbf{Input:} image $\mathbf{x}_v$, prompt $\mathbf{x}_t$, ground-truth $\mathbf{y}_t$; 
teacher modules $(V^T,P^T,L^T)$; 
student modules $(V^S,P^S,L^S)$; 
temperature $\tau$; loss weights $\lambda_1,\lambda_2$.\\
\textbf{Output:} \mbox{total training loss $\mathcal{L}$}.
\end{flushleft}
\begin{algorithmic}[1]
\STATE \textbf{\textit{// Standard Alignment Pathway}}
\STATE compute teacher logits $\mathbf{z}^T = L^T(P^T(V^T(\mathbf{x}_v)), \mathbf{x}_t)$
\STATE compute student logits $\mathbf{z}^S = L^S(P^S(V^S(\mathbf{x}_v)), \mathbf{x}_t)$
\STATE $\mathcal{L}_{\text{Align}} = \mathcal{L}_{\text{DBiLD}}(\mathbf{z}^T, \mathbf{z}^S)$

\STATE \textbf{\textit{// Visual-Switch Pathway}}
\STATE compute visual-switch logits \\
\hspace{1.2em}$\mathbf{z}^{Switch} = L^T(P^T(V^S(\mathbf{x}_v)), \mathbf{x}_t)$   
\STATE $\mathcal{L}_{\text{VSD}} = \mathcal{L}_{\text{DBiLD}}(\mathbf{z}^T, \mathbf{z}^{Switch})$

\STATE \textbf{\textit{// Language modeling objective}}
\STATE compute student next-token distribution \\
\hspace{1.2em}$\mathbf{p}^S = \mathrm{softmax}(\mathbf{z}^S / \tau)$
\STATE $\mathcal{L}_{\text{CE}} = -\sum_t \log \mathbf{p}^S(\mathbf{y}_t\,|\,\mathbf{x}_v, \mathbf{y}_{<t})$

\STATE \textbf{\textit{// Final objective}}
\STATE $\mathcal{L} = \mathcal{L}_{\text{CE}} + \lambda_1 \mathcal{L}_{\text{Align}} + \lambda_2 \mathcal{L}_{\text{VSD}}$
\STATE \textbf{return} $\mathcal{L}$
\end{algorithmic}
\end{algorithm}

\begin{algorithm}[htbp]
\caption{Calculation of DBiLD Loss}
\label{alg:dbild_calc}
\begin{flushleft}
\textbf{Input:} teacher logits $\mathbf{z}^t$, student logits $\mathbf{z}^s$.\\
\textbf{Output:} the DBiLD loss $\mathcal{L}_{\text{DBiLD}}$.
\end{flushleft}
\begin{algorithmic}[1]
\STATE \textbf{\textit{// Teacher-guided Loss}}

\STATE compute the transition point $k^t$ on sorted $\mathbf{z}^t$
\STATE select top-$k^t$ teacher logits $\mathbf{z}^t_{led}$
\STATE select corresponding student logits $\mathbf{z}^s_{cor}$
\STATE build pairwise differences $\mathbf{d}_{led}^{t}$ and $\mathbf{d}_{cor}^{s}$
\STATE normalize differences to probabilities $\mathbf{p}_{led}^{t}$ and $\mathbf{p}_{cor}^{s}$
\STATE $\mathcal{L}_t = D_{\text{RKL}}[\mathbf{p}_{led}^{t} \,\|\, \mathbf{p}_{cor}^{s}]$
\STATE \textbf{\textit{// Student-guided Loss}}
\STATE compute the transition point $k^s$ on sorted $\mathbf{z}^s$ 
\STATE select top-$k^s$ student logits $\mathbf{z}^s_{led}$ 
\STATE select corresponding teacher logits $\mathbf{z}^t_{cor}$
\STATE build pairwise differences $\mathbf{d}_{led}^{s}$ and $\mathbf{d}_{cor}^{t}$
\STATE normalize differences to probabilities $\mathbf{p}_{led}^{s}$ and $\mathbf{p}_{cor}^{t}$
\STATE $\mathcal{L}_s= D_{\text{RKL}}[\mathbf{p}_{cor}^{t} \,\|\, \mathbf{p}_{led}^{s}]$
\STATE \textbf{\textit{// Final objective}}
\STATE $\mathcal{L}_{\text{DBiLD}} = \mathcal{L}_t + \mathcal{L}_s$
\STATE \textbf{return} $\mathcal{L}_{\text{DBiLD}}$
\end{algorithmic}
\end{algorithm}

\section{Comparison with SOTA Distilled VLMs}
\paragraph{LLaVA-KD }
% \cite{cai2024llava} represents a state-of-the-art approach for VLM distillation, achieving konwledge transfer through explicit alignment from three dimensions: visual logits, language logits and self correlation matrix from the LLM-generated visual tokens.
\cite{cai2024llava} represents a state-of-the-art approach for VLM distillation, 
achieving knowledge transfer via explicit alignment of visual logits, language logits, and self-correlation matrices of LLM-generated visual tokens. 
We evaluate our method on the same benchmarks and training data as LLaVA-KD to ensure a fair comparison. 
Switch-KD achieves notable performance improvements at equivalent model scales, with average gains of 1.1 and 0.4 points for 0.5B and 1.5B student models, respectively. 
To further clarify the similarities and distinctions between the two methods, we summarize them below:
\begin{itemize}
    \item \textbf{Architecture Design.} 
    Similar to LLaVA-KD, Switch-KD maintains a simple yet effective architecture for the student VLM without introducing additional complexity or specialized modules.
    
    \item \textbf{Training Scheme.} 
    LLaVA-KD adopts a three-stage training framework comprising 
    (1) Distilled Pre-Training (DPT) for visual–textual alignment,(2) Supervised Fine-Tuning (SFT) for task-specific knowledge acquisition, and (3) Distilled Fine-Tuning (DFT) for teacher–student knowledge transfer. In contrast, our framework uses only standard Pre-Training (PT) followed by DFT with a visual-switch distillation design, effectively achieving both efficient knowledge acquisition and knowledge transfer, without introducing any additional training stages.
    
    \item \textbf{Distillation Strategy.} 
    LLaVA-KD employs dedicated knowledge distillation strategies (MDist/RDist) across both DPT and DFT stages.
    In contrast, Switch-KD introduces a dynamically attentive distillation mechanism through the proposed DBiLD loss during the DFT stage, enabling adaptive alignment of informative logits between teacher and student. 
    
\end{itemize}

\begin{figure*}[htbp]
    \centering
    \includegraphics[width=\linewidth]{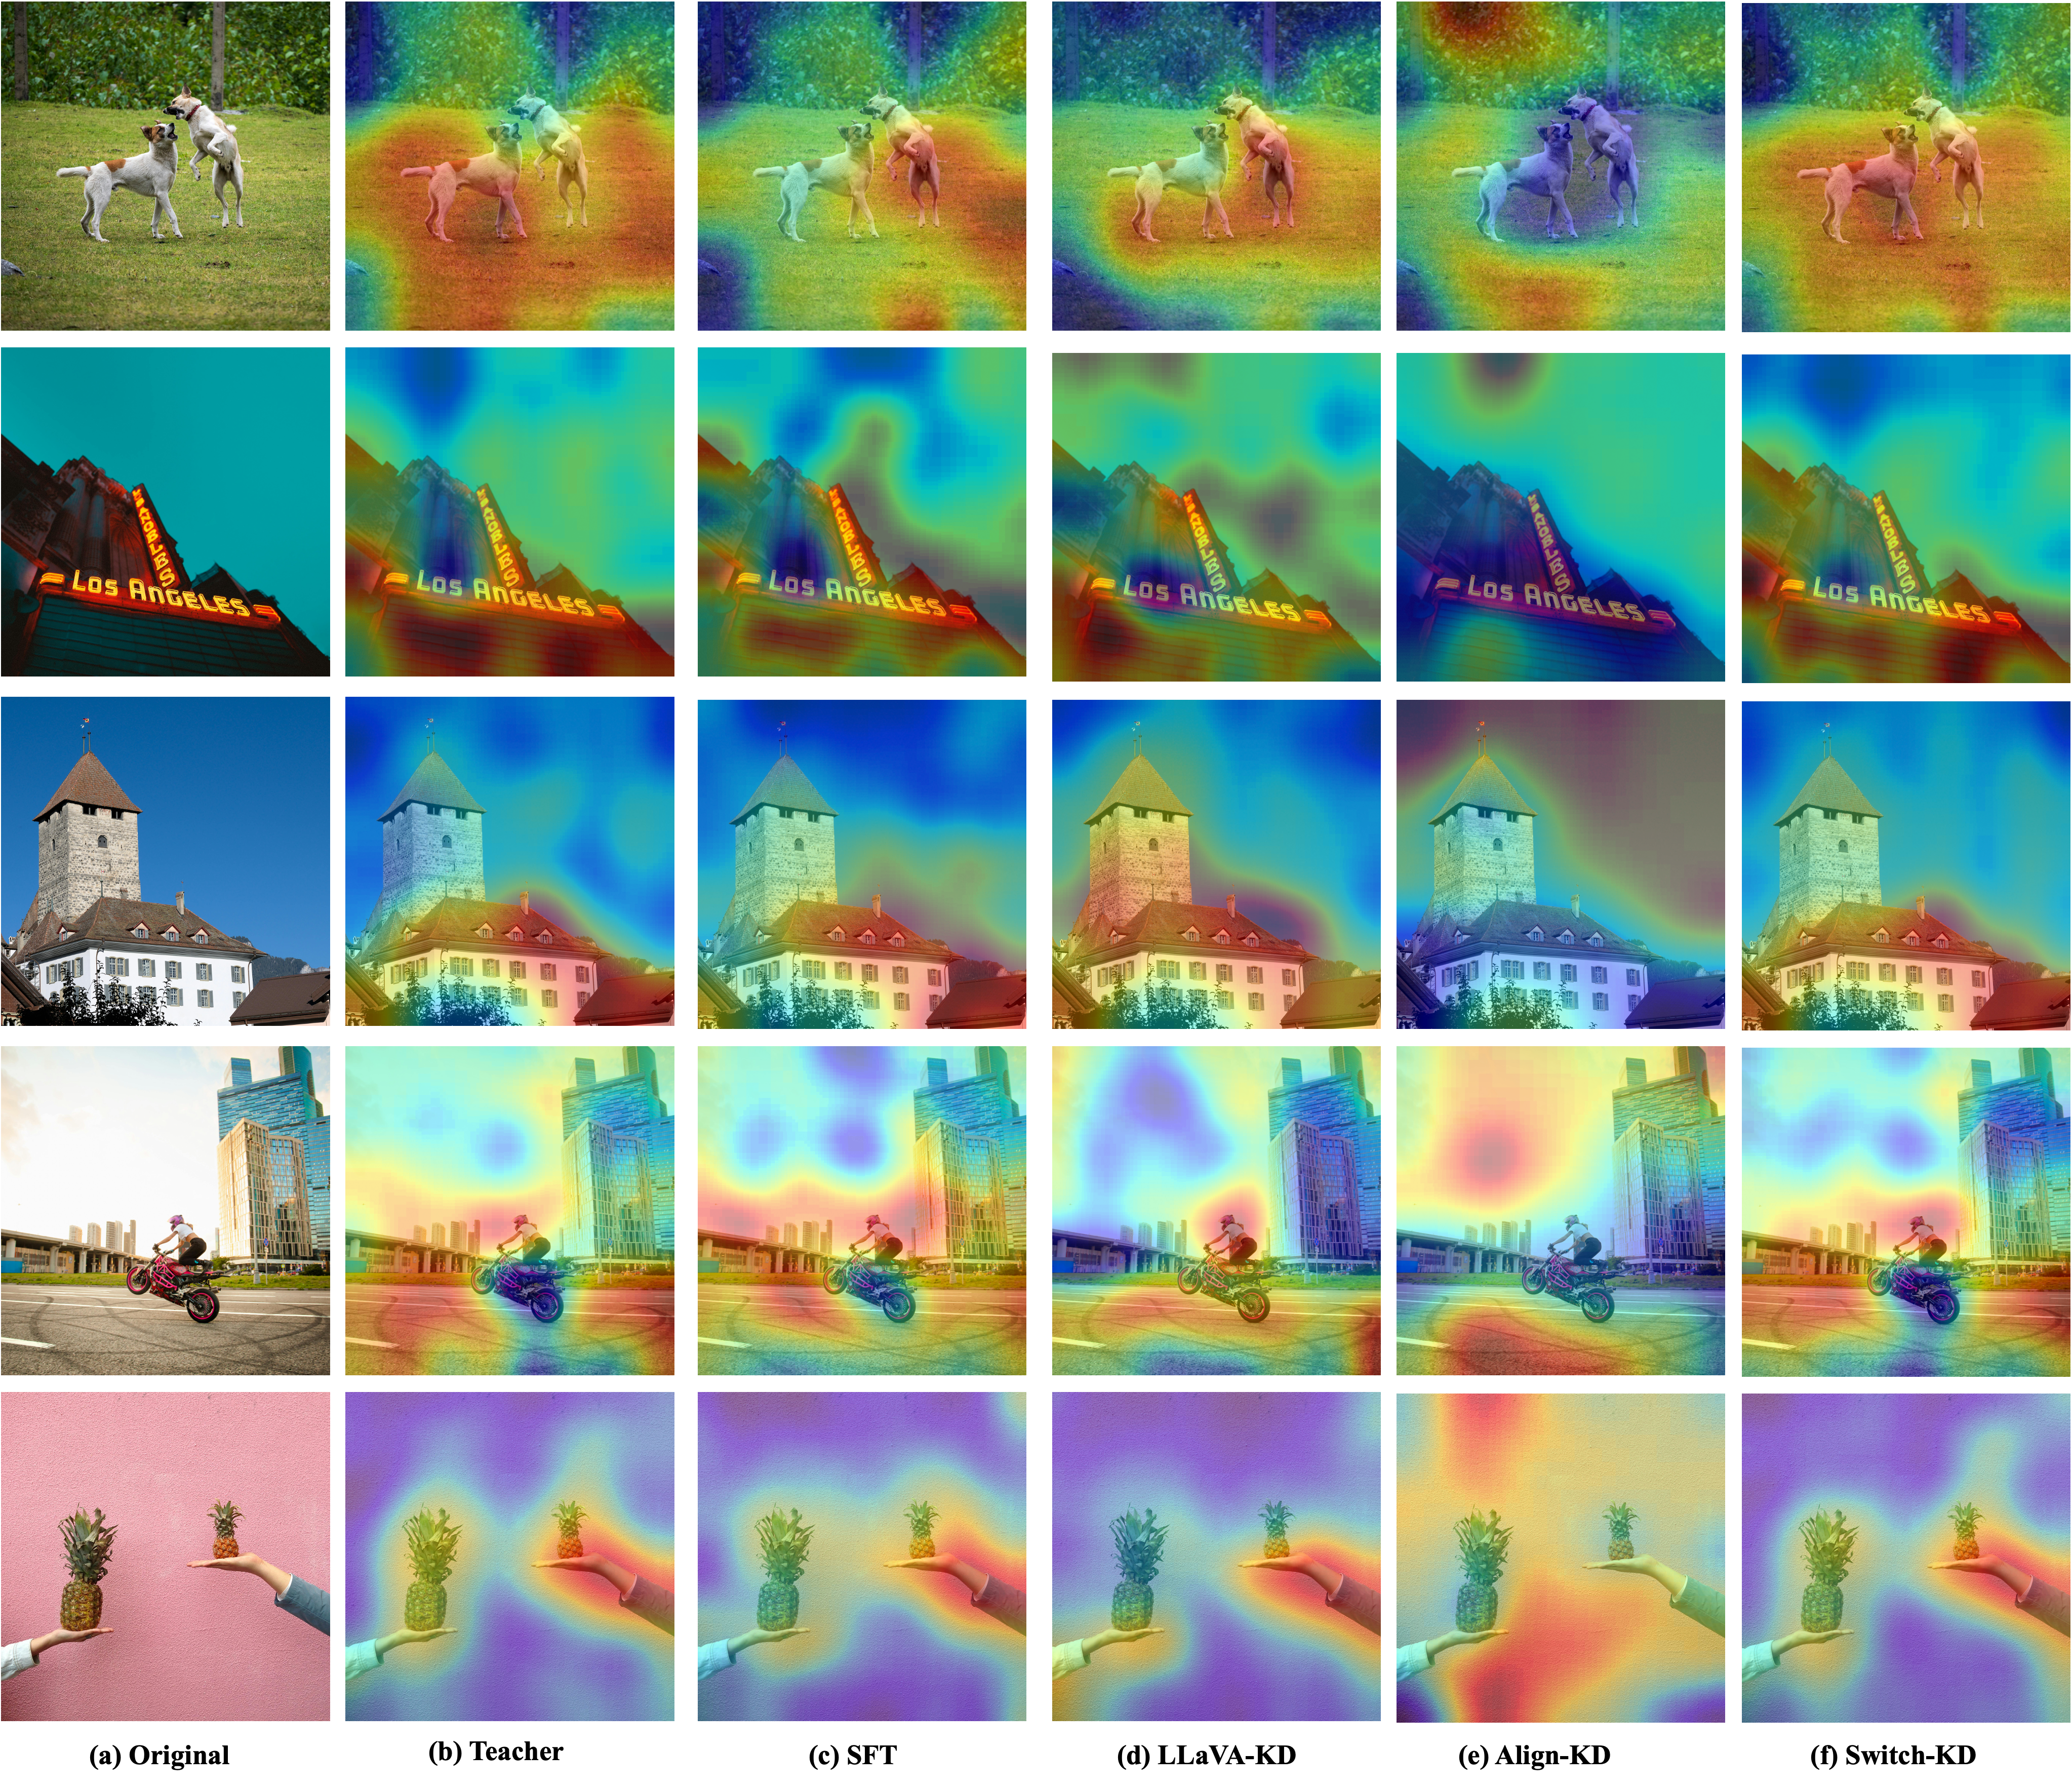}
    \caption{Visualization of attention maps for different distillation strategies.}
    \label{fig:app-attention}
\end{figure*}

\paragraph{Align-KD }
% \cite{feng2025align} represents another recent advance in multimodal distillation, introducing alignment constraints across three additional dimensions: cross-modal attention, visual tokens, and language logits.
\cite{feng2025align} is another recent advance in multimodal distillation, 
achieving knowledge transfer via explicit alignment of cross-modal attention, visual tokens, and language logits.
%\paragraph{Align-KD } \cite{feng2025align} is another recent effort in multimodal distillation, achieving knowledge transfer through explicit alignment across three dimensions: cross-modal attention, visual tokens, and language logits. 
We evaluate our approach on the same benchmarks as Align-KD, and despite using only about one-third of the training data (3M vs. 1.2M samples) and a lighter language backbone (1.7B vs. 1.5B parameters), Switch-KD achieves an average performance gain of 4.4 points.
To further highlight the similarities and differences between Align-KD and our approach, we summarize three key aspects below:

\begin{itemize}
    \item \textbf{Architecture Design.} 
    Both methods adopt similar vision–language model architectures, 
    while our approach employs a lighter LLM backbone, reducing computational cost without sacrificing performance.
    
    \item \textbf{Training Scheme.} 
    Both frameworks utilize a two-stage training paradigm in which distillation is introduced during the multi-task fine-tuning phase. 

    \item \textbf{Distillation Strategy.}
    Align-KD distills knowledge from the text-query–vision part of the first attention layer and selectively, although unevenly, enhances vision tokens based on the attention focus of text tokens. In contrast, our method performs unified and adaptive multimodal alignment across the entire output distribution via the proposed DBiLD loss.
\end{itemize}
    
% \section{Visualization of attention maps}

\begin{table*}[htbp]
\centering
\setlength{\tabcolsep}{4pt}

\begin{tabular}{lccccccccccc}
\toprule
\multirow{2}{*}{\textbf{Training Strategy}} & 
\multicolumn{3}{c}{\textbf{Percep. \& Underst.}} &
\multicolumn{4}{c}{\textbf{Cognition \& Reasoning}} &
\multicolumn{1}{c}{\textbf{OCR}} &
\multicolumn{1}{c}{\textbf{Specific}} &
\multicolumn{1}{c}{\textbf{Halluc.}} &
\multirow{2}{*}{\textbf{Avg\textsubscript{10}}}\\
\cmidrule(lr){2-4}\cmidrule(lr){5-8}\cmidrule(lr){9-9}\cmidrule(lr){10-10}\cmidrule(lr){11-11}
& MME & MMB & MMB$^{\text{CN}}$ & VQAv2 & GQA & SciQA & MMMU & TextVQA & VizWiz & POPE & \\
\midrule
\textbf{PT+SFT ($V^S$)}
& 61.5 & 58.9 & 54.2 & 74.8 & 58.3 & \textbf{59.1} & \textbf{33.6} & 49.2 & 28.9 & 86.1 & 56.5 \\

\textbf{PT+SFT ($V^T$)}
& 62.0 & 55.2 & 51.3 & 75.7 & 58.0 & 57.9 & 29.7 & 44.7 & 41.3 & 84.6 & 56.0 \\

\rowcolor{green!10}
\textbf{Switch-KD}
& \textbf{66.8} & \textbf{63.5} & \textbf{57.8} & \textbf{79.6} & \textbf{61.6} & 57.9 & 29.8 & \textbf{52.3} & \textbf{44.9} & \textbf{87.3} & \textbf{60.1} \\
\bottomrule
\end{tabular}
\caption{
Ablation study on direct visual encoder substitution. 
\textbf{PT+SFT ($V^S$)} denotes standard pre-training (PT) and supervised fine-tuning (SFT) with the original visual encoder $V^S$. 
\textbf{PT+SFT ($V^T$)} denotes the same PT+SFT pipeline but with the teacher visual encoder $V^T$ replacing $V^S$. 
\textbf{Switch-KD} denotes pre-training followed by distilled fine-tuning (DFT) with the proposed visual-switch distillation. 
Simply substituting $V^T$ does not outperform the baseline, whereas Switch-KD consistently achieves superior performance.
}
\label{tab:teacherenc}
\end{table*}

\begin{table*}[htbp]
\centering
\setlength{\tabcolsep}{4pt}

\begin{tabular}{lccccccccccc}
\toprule
\multirow{2}{*}{\textbf{Training Scheme}} & 
\multicolumn{3}{c}{\textbf{Percep. \& Underst.}} &
\multicolumn{4}{c}{\textbf{Cognition \& Reasoning}} &
\multicolumn{1}{c}{\textbf{OCR}} &
\multicolumn{1}{c}{\textbf{Specific}} &
\multicolumn{1}{c}{\textbf{Halluc.}} &
\multirow{2}{*}{\textbf{Avg\textsubscript{10}}}\\
\cmidrule(lr){2-4}\cmidrule(lr){5-8}\cmidrule(lr){9-9}\cmidrule(lr){10-10}\cmidrule(lr){11-11}
& MME & MMB & MMB$^{\text{CN}}$ & VQAv2 & GQA & SciQA & MMMU & TextVQA & VizWiz & POPE & \\
\midrule
PT-SFT   & 61.5 & 58.9 & 54.2 & 74.8 & 58.3 & \textbf{59.1} & \textbf{33.6} & 49.2 & 28.9 & 86.1 & 56.5 \\
DPT-SFT  & \textbf{65.6} & 57.4 & 53.2 & 76.5 & 58.6 & 58.4 & 32.2 & 50.2 & 35.4 & 86.8 & 57.4 \\
\rowcolor{blue!10}
PT-DFT   & 63.1 & \textbf{60.8} & 57.3 & \textbf{77.8} & \textbf{59.7} & 58.1 & 31.7 & 51.0 & \textbf{41.5} & \textbf{87.0} & \textbf{58.8} \\
DPT-DFT  & 63.6 & 60.5 & \textbf{57.4} & 77.2 & 59.6 & 58.2 & 32.0 & \textbf{51.1} & 41.4 & 86.4 & 58.7 \\
\bottomrule
\end{tabular}
\caption{
Ablation study on different training schemes.
}
\label{tab:scheme}
\end{table*}

\begin{table*}[h]
\centering
\setlength{\tabcolsep}{4pt}

\begin{tabular}{ccccccccccccc}
\toprule
\multirow{2}{*}{\textbf{Teacher}} & 
\multirow{2}{*}{\textbf{Student}} &
% \multirow{2}{*}{\shortstack{\textbf{Teacher}\\\textbf{LLM}}} &
% \multirow{2}{*}{\shortstack{\textbf{Student}\\\textbf{LLM}}} &
\multicolumn{3}{c}{\textbf{Percep. \& Underst.}} &
\multicolumn{4}{c}{\textbf{Cognition \& Reasoning}} &
\multicolumn{1}{c}{\textbf{OCR}} &
\multicolumn{1}{c}{\textbf{Specific}} &
\multicolumn{1}{c}{\textbf{Halluc.}} &
\multirow{2}{*}{\textbf{Avg\textsubscript{10}}}\\
\cmidrule(lr){3-5}\cmidrule(lr){6-9}\cmidrule(lr){10-10}\cmidrule(lr){11-11}\cmidrule(lr){12-12}
& & MME & MMB & MMB$^{\text{CN}}$ & VQAv2 & GQA & SciQA & MMMU & TextVQA & VizWiz & POPE & \\
\midrule
7B  & \multirow{2}{*}{/} & 77.4 & 74.9 & 74.4 & 81.3 & 64.0 & 73.6 & 41.6 & 60.3 & 53.9 & 86.8 &68.8 \\
3B  &  & 73.9 & 71.8 & 69.5 & 80.4 & 63.2 & 76.0 & 40.3 & 61.5 & 38.7 & 86.4 & 66.2 \\
\midrule
/  & 1.5B & 72.5 & 68.6 & 63.0 & 78.8 & 62.0 & \textbf{72.0} & \textbf{37.0} & 57.4 & 43.2 & 85.5 & 64.0 \\
\rowcolor{blue!10}
7B  & 1.5B & 72.2 & 71.4 & \textbf{68.5} &\textbf{81.4}&\textbf{63.9} &69.3&34.9&\textbf{60.3}&\textbf{44.4}&86.8&\textbf{65.3} \\
3B  & 1.5B & \textbf{72.6} & \textbf{72.2} & 68.3 & 80.6 & 62.2 & 70.0 & 33.9 & 59.1 & 42.5 & \textbf{86.9} & 64.8 \\
\midrule
/  & 0.5B & 61.5 & 58.9 & 54.2 & 74.8 & 58.3 & \textbf{59.1} & \textbf{33.6} & 49.2 & 28.9 & 86.1 & 56.5 \\
7B  & 0.5B & 66.1 & 61.6 & 56.9 & \textbf{79.7} & \textbf{62.1} & 58.1 & 31.2 & \textbf{52.6} & 42.6 & 87.0 & 59.8 \\
\rowcolor{blue!10}
3B  & 0.5B & \textbf{66.8}&\textbf{63.5}&\textbf{57.8}&79.6&61.6&57.9&29.8&52.3&\textbf{44.9}&\textbf{87.3}&\textbf{60.1} \\
\bottomrule
\end{tabular}
\caption{
Ablation study on teacher models with different sizes.
}
\label{tab:teacher_scale}
\end{table*}
\section{More Ablation and Explanatory Analysis}
\label{ablation}
\subsection{More Visualization of Attention Maps}
\label{attenmap}
Fig.~\ref{fig:app-attention} presents additional qualitative comparisons of visual attention across five representative image pairs. 
The teacher model consistently focuses on semantically critical regions that closely correspond to the textual queries. 
The SFT baseline produces diffuse and unstable attention, often failing to localize salient regions or spreading attention across large background areas, indicating insufficient visual grounding.
LLaVA-KD mainly focuses on key semantic regions, but still exhibits noisy patches and inconsistent localization across images.
%LLaVA-KD improves overall focus but still exhibits noisy patches and inconsistent localization across images, suggesting limited ability to transfer the teacher’s fine-grained visual cues. 
Align-KD tends to focus on background regions rather than key objects, resulting in overly diffuse attention.
%Our Switch-KD effectively reconstructs this fine-grained attention pattern, capturing key visual cues that are well aligned with semantics.
Across all examples, Our Switch-KD maintains stable object-centric focus and effectively reconstructs the teacher's fine-grained attention pattern, demonstrating that its visual-switch architecture and dynamic logit selection effectively guides the student to learn more faithful and interpretable visual representations.

\subsection{Further Validation of the Visual-Switch Hypothesis}
We formulated the core hypothesis that if the student visual encoder $V^S$ learns meaningful representations, 
its visual features should be correctly interpreted and decoded by the teacher’s language pathway, 
yielding a probability distribution consistent with the teacher’s original output. 
A natural follow-up question is whether the performance could be improved simply by replacing the student visual encoder with the teacher’s visual encoder, thereby starting PT and SFT with higher-quality visual representations.
To investigate this, we conduct an experiment where the student model is initialized with the teacher’s visual encoder and trained under the standard PT+SFT paradigm. 
Surprisingly, as shown in Table~\ref{tab:teacherenc}, this direct substitution not only fails to surpass the baseline performance, but in some cases even performs worse—despite the teacher encoder providing substantially stronger visual representations. This indicates that simply transplanting a high-capacity encoder does not guarantee effective knowledge transfer, likely due to representational mismatches between the teacher’s visual features and the student’s language pathway, as well as the absence of explicit alignment signals during PT and SFT.
In contrast, our proposed Switch-KD consistently yields notable improvements. 
These results suggest that Switch-KD achieves a well-balanced integration: effectively learning the teacher’s visual knowledge while aligning it with the student’s language backbone through unified text-probability supervision.

\section{Detailed Results}
\subsection{Ablation Study on Training Schemes}
Table~\ref{tab:scheme} shows more detailed results of the ablation study on different training schemes, including PT-SFT, DPT-SFT, PT-DFT and DPT-DFT.
DFT–SFT notably improves the student model’s performance on the MME and VizWiz datasets, but the overall gain remains limited. PT–DFT outperforms PT–SFT by 2.3 point, indicating that DFT contributes more than SFT to downstream performance. DPT–DFT achieves results largely comparable to PT–SFT across all datasets, suggesting that the performance improvements mainly stem from DFT. Therefore, we adopt the PT–DFT training scheme to ensure an efficient and effective training paradigm.

\subsection{Ablation study on Teacher's Size}
Table~\ref{tab:teacher_scale} shows more detailed results of the ablation study that investigates the impact of different teacher sizes. Across all teacher sizes, Switch-KD consistently improves performance, indicating that it effectively transfers useful knowledge while mitigating teacher–student mismatch.
For the 1.5B student, larger teachers lead to higher accuracy: the 7B teacher achieves the best overall score of 65.3, outperforming both the 3B teacher the no-teacher baseline. This shows that stronger teachers provide richer supervisory signals, especially for reasoning-heavy tasks such as VQAv2 and SciQA.
For the 0.5B student, distilling from a 3B or 7B teacher yields clear improvements over the baseline, with the 3B teacher slightly outperforming the 7B teacher. This suggests a capacity–compatibility effect: extremely large teachers may produce representations too difficult for very small students to fully understand.
